# Supplementary material for: OOD Aware Supervised Contrastive Learning
Source: arXiv:2310.01942 source file (2023-10-03)
Supplement: Supplementary file 1 [file other-ood.tex]

\begin{table*}
\scriptsize
\centering
\setlength{\extrarowheight}{0pt}
\addtolength{\extrarowheight}{\aboverulesep}
\addtolength{\extrarowheight}{\belowrulesep}
\setlength{\aboverulesep}{0pt}
\setlength{\belowrulesep}{0pt}
\begin{tabular}{|p{1.1cm}|p{0.6cm}|p{0.6cm}|p{\metricsize}|p{\metricsize}|p{\metricsize}|p{\metricsize}|p{\metricsize}|p{\metricsize}|p{\metricsize}|p{\metricsize}|p{\metricsize}|p{\metricsize}|p{\metricsize}|p{\metricsize}|} 
\toprule
Dataset  & \begin{sideways}Accuracy\end{sideways}  & Metric &\begin{sideways}DTD\end{sideways} & \multicolumn{1}{|l|}{\begin{sideways}SVHN\end{sideways}} & \multicolumn{1}{l|}{\begin{sideways}Places365\end{sideways}} & \multicolumn{1}{l|}{\begin{sideways}LSUN-C\end{sideways}} & \multicolumn{1}{l|}{\begin{sideways}LSUN-R\end{sideways}} & \multicolumn{1}{l|}{\begin{sideways}iSUN\end{sideways}} &  \multicolumn{1}{l|}{\begin{sideways}iNaturalist\end{sideways}} & \multicolumn{1}{l|}{\begin{sideways}CIFAR-100\end{sideways}} & \multicolumn{1}{l|}{\begin{sideways}MNIST\end{sideways}} & \multicolumn{1}{l|}{\begin{sideways}TIN\end{sideways}} & \begin{sideways}Average\end{sideways}  \\ 
\hline
\hline

\multirow{3}{*}{\Longunderstack{TIM}} &
\multirow{3}{*}{95.31} & % Accuracy
{\cellcolor{\fprcolor}}{\tiny FPR$\downarrow$} &
{\cellcolor{\fprcolor}} 19.54 & {\cellcolor{\fprcolor}} 2.01 & {\cellcolor{\fprcolor}} 21.54 & {\cellcolor{\fprcolor}} 1.02 & {\cellcolor{\fprcolor}} 9.06 & {\cellcolor{\fprcolor}} 11.65 & {\cellcolor{\fprcolor}} 25.40 & {\cellcolor{\fprcolor}} 38.20 & {\cellcolor{\fprcolor}} 0.56 & {\cellcolor{\fprcolor}} 27.52 & {\cellcolor{\fprcolor}} 15.65  \\

& & {\cellcolor{\auroccolor}}{\tiny AUROC$\uparrow$} &
{\cellcolor{\auroccolor}} 96.65 & {\cellcolor{\auroccolor}} 99.56 & {\cellcolor{\auroccolor}} 95.48 & {\cellcolor{\auroccolor}} 99.60 & {\cellcolor{\auroccolor}} 98.16 & {\cellcolor{\auroccolor}} 97.80 & {\cellcolor{\auroccolor}} 95.46 & {\cellcolor{\auroccolor}} 92.58 & {\cellcolor{\auroccolor}} 99.82 & {\cellcolor{\auroccolor}} 93.64 & {\cellcolor{\auroccolor}} 96.87 \\

& & {\cellcolor{\auprcolor}}{\tiny AUPR$\uparrow$} &
{\cellcolor{\auprcolor}} 98.17 & {\cellcolor{\auprcolor}} 99.00 & {\cellcolor{\auprcolor}} 50.35 & {\cellcolor{\auprcolor}} 99.64 & {\cellcolor{\auprcolor}} 98.49 & {\cellcolor{\auprcolor}} 98.34 & {\cellcolor{\auprcolor}} 81.37 & {\cellcolor{\auprcolor}} 92.63 & {\cellcolor{\auprcolor}} 99.83& {\cellcolor{\auprcolor}} 92.97 & {\cellcolor{\auprcolor}} 91.07 \\ 

\hline

\multirow{3}{*}{SVHN} & 
\multirow{3}{*}{95.47} & % Accuracy
{\cellcolor{\fprcolor}}{\tiny FPR$\downarrow$}
& {\cellcolor{\fprcolor}} 13.05 & {\cellcolor{\fprcolor}} 4.89 & {\cellcolor{\fprcolor}} 20.73 & {\cellcolor{\fprcolor}} 0.42 & {\cellcolor{\fprcolor}} 6.39 & {\cellcolor{\fprcolor}} 6.85  & {\cellcolor{\fprcolor}} 20.53 & {\cellcolor{\fprcolor}} 38.95 & {\cellcolor{\fprcolor}} 0.68 & {\cellcolor{\fprcolor}} 27.34 & {\cellcolor{\fprcolor}} 13.98 \\

& & {\cellcolor{\auroccolor}}{\tiny AUROC$\uparrow$} & 
{\cellcolor{\auroccolor}} 97.61 & {\cellcolor{\auroccolor}} 99.07 & {\cellcolor{\auroccolor}} 95.76 & {\cellcolor{\auroccolor}} 99.80 & {\cellcolor{\auroccolor}} 98.62 & {\cellcolor{\auroccolor}}  98.58 & {\cellcolor{\auroccolor}} 96.28 & {\cellcolor{\auroccolor}} 92.61 & {\cellcolor{\auroccolor}} 99.73 & {\cellcolor{\auroccolor}} 93.87 & {\cellcolor{\auroccolor}} 97.19 \\

& & {\cellcolor{\auprcolor}}{\tiny AUPR$\uparrow$}  & 
{\cellcolor{\auprcolor}} 98.64 & {\cellcolor{\auprcolor}} 98.01 & {\cellcolor{\auprcolor}} 51.07 & {\cellcolor{\auprcolor}} 99.81 & {\cellcolor{\auprcolor}} 98.84 & {\cellcolor{\auprcolor}} 98.91 & {\cellcolor{\auprcolor}} 82.92 & {\cellcolor{\auprcolor}} 92.64 & {\cellcolor{\auprcolor}} 99.75 & {\cellcolor{\auprcolor}} 93.16 & {\cellcolor{\auprcolor}} 91.37 \\  

\hline

\multirow{3}{*}{Textures} 
& \multirow{3}{*}{95.44} % Accuracy
& {\cellcolor{\fprcolor}}{\tiny FPR$\downarrow$}   
& {\cellcolor{\fprcolor}} 18.00 & {\cellcolor{\fprcolor}} 1.86 & {\cellcolor{\fprcolor}} 20.98 & {\cellcolor{\fprcolor}} 0.70 & {\cellcolor{\fprcolor}} 6.16 & {\cellcolor{\fprcolor}} 7.37  & {\cellcolor{\fprcolor}} 24.35 & {\cellcolor{\fprcolor}} 38.86 & {\cellcolor{\fprcolor}} 0.40 & {\cellcolor{\fprcolor}} 27.58 & {\cellcolor{\fprcolor}} 14.62  \\

& & {\cellcolor{\auroccolor}}{\tiny AUROC$\uparrow$} & 
{\cellcolor{\auroccolor}} 97.07 & {\cellcolor{\auroccolor}} 99.62 & {\cellcolor{\auroccolor}} 95.68 & {\cellcolor{\auroccolor}} 99.72 & {\cellcolor{\auroccolor}} 98.67 & {\cellcolor{\auroccolor}} 98.53 & {\cellcolor{\auroccolor}} 95.69 & {\cellcolor{\auroccolor}} 92.66 & {\cellcolor{\auroccolor}} 99.89 & {\cellcolor{\auroccolor}} 93.76 & {\cellcolor{\auroccolor}} 97.12 \\

& &{\cellcolor{\auprcolor}}{\tiny AUPR$\uparrow$}  & 
{\cellcolor{\auprcolor}} 98.41 & {\cellcolor{\auprcolor}} 99.10 & {\cellcolor{\auprcolor}} 49.98 & {\cellcolor{\auprcolor}} 99.74 & {\cellcolor{\auprcolor}} 98.89 & {\cellcolor{\auprcolor}} 98.88 & {\cellcolor{\auprcolor}} 81.22 & {\cellcolor{\auprcolor}} 92.68 & {\cellcolor{\auprcolor}} 99.89 & {\cellcolor{\auprcolor}} 92.94 & {\cellcolor{\auprcolor}} 91.17 \\  

\hline

\multirow{3}{*}{iNaturalist} & 
\multirow{3}{*}{95.33} & % Accuracy
{\cellcolor{\fprcolor}}{\tiny FPR$\downarrow$} & {\cellcolor{\fprcolor}} 13.99 & {\cellcolor{\fprcolor}} 1.76 & {\cellcolor{\fprcolor}} 22.17  & {\cellcolor{\fprcolor}} 0.40  & {\cellcolor{\fprcolor}} 5.59  & {\cellcolor{\fprcolor}} 5.99  & {\cellcolor{\fprcolor}} 18.82 & {\cellcolor{\fprcolor}} 38.39 & {\cellcolor{\fprcolor}} 0.58 & {\cellcolor{\fprcolor}} 27.58 & {\cellcolor{\fprcolor}} 13.52  \\

& & {\cellcolor{\auroccolor}}{\tiny AUROC$\uparrow$} & 
{\cellcolor{\auroccolor}} 97.48 & {\cellcolor{\auroccolor}} 99.62 & {\cellcolor{\auroccolor}} 95.40  & {\cellcolor{\auroccolor}} 99.81 & {\cellcolor{\auroccolor}} 98.72 & {\cellcolor{\auroccolor}} 98.66 & {\cellcolor{\auroccolor}} 96.44 & {\cellcolor{\auroccolor}} 92.56 & {\cellcolor{\auroccolor}} 99.84 & {\cellcolor{\auroccolor}} 93.62 & {\cellcolor{\auroccolor}} 97.21 \\

& & {\cellcolor{\auprcolor}}{\tiny AUPR$\uparrow$}  & 
{\cellcolor{\auprcolor}} 98.59 & {\cellcolor{\auprcolor}} 99.12 & {\cellcolor{\auprcolor}} 49.08 & {\cellcolor{\auprcolor}} 
99.82 & {\cellcolor{\auprcolor}} 98.93 & {\cellcolor{\auprcolor}} 98.98 & {\cellcolor{\auprcolor}} 83.41 & {\cellcolor{\auprcolor}} 92.56 & {\cellcolor{\auprcolor}} 99.84 & {\cellcolor{\auprcolor}} 92.82 & {\cellcolor{\auprcolor}} 91.31 \\

\hline

\multirow{3}{*}{Places365} &
\multirow{3}{*}{95.39} & % Accuracy
{\cellcolor{\fprcolor}}{\tiny FPR$\downarrow$} &
{\cellcolor{\fprcolor}} 20.07 & {\cellcolor{\fprcolor}} 1.78 & {\cellcolor{\fprcolor}} 21.84  & {\cellcolor{\fprcolor}} 0.51  & {\cellcolor{\fprcolor}} 8.42  & {\cellcolor{\fprcolor}} 10.42  & {\cellcolor{\fprcolor}} 26.57 & {\cellcolor{\fprcolor}} 39.99 & {\cellcolor{\fprcolor}} 0.52 & {\cellcolor{\fprcolor}} 29.06 & {\cellcolor{\fprcolor}} 15.91  \\

& & {\cellcolor{\auroccolor}}{\tiny AUROC$\uparrow$} & 
{\cellcolor{\auroccolor}} 96.67 & {\cellcolor{\auroccolor}} 99.64 & {\cellcolor{\auroccolor}} 95.55  & {\cellcolor{\auroccolor}}  99.79 & {\cellcolor{\auroccolor}} 98.31 & {\cellcolor{\auroccolor}} 98.05 & {\cellcolor{\auroccolor}} 95.40 & {\cellcolor{\auroccolor}} 92.40 & {\cellcolor{\auroccolor}} 99.85 & {\cellcolor{\auroccolor}} 93.51 & {\cellcolor{\auroccolor}} 96.91 \\

& & {\cellcolor{\auprcolor}}{\tiny AUPR$\uparrow$}  & 
{\cellcolor{\auprcolor}} 98.16 & {\cellcolor{\auprcolor}} 99.14 & {\cellcolor{\auprcolor}} 50.10 & {\cellcolor{\auprcolor}} 
99.80 & {\cellcolor{\auprcolor}} 98.61 & {\cellcolor{\auprcolor}} 98.52 & {\cellcolor{\auprcolor}} 80.83 & {\cellcolor{\auprcolor}} 92.48 & {\cellcolor{\auprcolor}} 99.85 & {\cellcolor{\auprcolor}} 92.79 & {\cellcolor{\auprcolor}} 91.72 \\

\bottomrule
\end{tabular}
\caption {\textbf{Results obtained with ResNet18 and CIFAR-10 dataset as the ID data for different OOD datasets used for training. For each method we report three metrics: \FPR$\downarrow$, \AUROC$\uparrow$ and \AUPR$\uparrow$}. The first column denotes the classification accuracy on the ID dataset.}
\label{tab:other_ood}
\end{table*}
