# Supplementary material for: OOD Aware Supervised Contrastive Learning
Source: arXiv:2310.01942 source file (2023-10-03)
Supplement: Supplementary file 3 [file FTvsScratch.tex]

\begin{table*}
\scriptsize
\centering
\setlength{\extrarowheight}{0pt}
\addtolength{\extrarowheight}{\aboverulesep}
\addtolength{\extrarowheight}{\belowrulesep}
\setlength{\aboverulesep}{0pt}
\setlength{\belowrulesep}{0pt}
\begin{tabular}{|p{1.1cm}|p{0.6cm}|p{0.6cm}|p{\metricsize}|p{\metricsize}|p{\metricsize}|p{\metricsize}|p{\metricsize}|p{\metricsize}|p{\metricsize}|p{\metricsize}|p{\metricsize}|p{\metricsize}|p{\metricsize}|} 
\toprule
Method &\begin{sideways}Accuracy\end{sideways} & Metric &\begin{sideways}DTD\end{sideways} & \multicolumn{1}{|l|}{\begin{sideways}SVHN\end{sideways}} & \multicolumn{1}{l|}{\begin{sideways}Places365\end{sideways}} & \multicolumn{1}{l|}{\begin{sideways}LSUN-C\end{sideways}} & \multicolumn{1}{l|}{\begin{sideways}LSUN-R\end{sideways}} & \multicolumn{1}{l|}{\begin{sideways}iSUN\end{sideways}} &  \multicolumn{1}{l|}{\begin{sideways}iNaturalist\end{sideways}} & \multicolumn{1}{l|}{\begin{sideways}CIFAR-100\end{sideways}} & \multicolumn{1}{l|}{\begin{sideways}MNIST\end{sideways}} & \multicolumn{1}{l|}{\begin{sideways}TIN\end{sideways}} & \begin{sideways}Average\end{sideways}  \\ 
\hline
\hline

\multirow{3}{*}{\Longunderstack{OPSupCon \\ \tiny (Real-OOD) \\ AA \\ Finetune}}& 
\multirow{3}{*}{95.31} & % Accuracy
{\cellcolor{\fprcolor}}{\tiny FPR$\downarrow$} &
{\cellcolor{\fprcolor}} 19.54 & {\cellcolor{\fprcolor}} 2.01 & {\cellcolor{\fprcolor}} 21.54 & {\cellcolor{\fprcolor}} 1.02 & {\cellcolor{\fprcolor}} 9.06 & {\cellcolor{\fprcolor}} 11.65 & {\cellcolor{\fprcolor}} 25.40 & {\cellcolor{\fprcolor}} 38.20 & {\cellcolor{\fprcolor}} 0.56 & {\cellcolor{\fprcolor}} 27.52 & {\cellcolor{\fprcolor}} 15.65  \\

& & {\cellcolor{\auroccolor}}{\tiny AUROC$\uparrow$} &
{\cellcolor{\auroccolor}} 96.65 & {\cellcolor{\auroccolor}} 99.56 & {\cellcolor{\auroccolor}} 95.48 & {\cellcolor{\auroccolor}} 99.60 & {\cellcolor{\auroccolor}} 98.16 & {\cellcolor{\auroccolor}} 97.80 & {\cellcolor{\auroccolor}} 95.46 & {\cellcolor{\auroccolor}} 92.58 & {\cellcolor{\auroccolor}} 99.82 & {\cellcolor{\auroccolor}} 93.64 & {\cellcolor{\auroccolor}} 96.87\\

& & {\cellcolor{\auprcolor}}{\tiny AUPR$\uparrow$} &
{\cellcolor{\auprcolor}} 98.17 & {\cellcolor{\auprcolor}} 99.00 & {\cellcolor{\auprcolor}} 50.35 & {\cellcolor{\auprcolor}} 99.64 & {\cellcolor{\auprcolor}} 98.49 & {\cellcolor{\auprcolor}} 98.34 & {\cellcolor{\auprcolor}} 81.37 & {\cellcolor{\auprcolor}} 92.63 & {\cellcolor{\auprcolor}} 99.83& {\cellcolor{\auprcolor}} 92.97 & {\cellcolor{\auprcolor}} 91.07 \\ 

\hline

\multirow{3}{*}{\Longunderstack{OPSupCon \\ \tiny (Real-OOD) \\ AA \\ Scratch}} & 
\multirow{3}{*}{95.43} & % Accuracy
{\cellcolor{\fprcolor}}{\tiny FPR$\downarrow$} & {\cellcolor{\fprcolor}} 17.20 & {\cellcolor{\fprcolor}} 4.92 & {\cellcolor{\fprcolor}} 25.42 & {\cellcolor{\fprcolor}} 2.93 & {\cellcolor{\fprcolor}} 4.78 & {\cellcolor{\fprcolor}} 4.92  & {\cellcolor{\fprcolor}} 22.43 & {\cellcolor{\fprcolor}} 43.21 & {\cellcolor{\fprcolor}} 2.45 & {\cellcolor{\fprcolor}} 31.31 & {\cellcolor{\fprcolor}} 15.95  \\

& & {\cellcolor{\auroccolor}}{\tiny AUROC$\uparrow$} & 
{\cellcolor{\auroccolor}} 96.21 & {\cellcolor{\auroccolor}} 99.00 & {\cellcolor{\auroccolor}} 94.83 & {\cellcolor{\auroccolor}} 99.19 & {\cellcolor{\auroccolor}} 98.81 & {\cellcolor{\auroccolor}} 98.78 & {\cellcolor{\auroccolor}} 95.79 & {\cellcolor{\auroccolor}} 91.08 & {\cellcolor{\auroccolor}} 99.41 & {\cellcolor{\auroccolor}} 93.11 & {\cellcolor{\auroccolor}} 96.62\\

& & {\cellcolor{\auprcolor}}{\tiny AUPR$\uparrow$}  & 
{\cellcolor{\auprcolor}} 97.49 & {\cellcolor{\auprcolor}} 97.80 & {\cellcolor{\auprcolor}} 47.46 & {\cellcolor{\auprcolor}} 99.30 & {\cellcolor{\auprcolor}} 99.02 & {\cellcolor{\auprcolor}} 99.08 & {\cellcolor{\auprcolor}} 80.88 & {\cellcolor{\auprcolor}} 91.23 & {\cellcolor{\auprcolor}} 99.47 & {\cellcolor{\auprcolor}} 92.46 & {\cellcolor{\auprcolor}} 91.11 \\  

\bottomrule
\end{tabular}
\caption {\textbf{Finetuning compared to training from scratch on CIFAR-10 dataset with a ResNet18 backbone.} For each method we report three metrics: \FPR$\downarrow$, \AUROC$\uparrow$ and \AUPR$\uparrow$. The first column denotes the classification accuracy on the ID dataset.}
\label{tab:ftvssc}
\end{table*}
