# Supplementary material for: OOD Aware Supervised Contrastive Learning
Source: arXiv:2310.01942 source file (2023-10-03)
Supplement: Supplementary file 4 [file mixed_cifar100.tex]

\begin{table}
\scriptsize
\centering
\setlength{\extrarowheight}{0pt}
\addtolength{\extrarowheight}{\aboverulesep}
\addtolength{\extrarowheight}{\belowrulesep}
\setlength{\aboverulesep}{0pt}
\setlength{\belowrulesep}{0pt}
\begin{tabular}{|p{1.1cm}|p{0.6cm}|p{\metricsize}p{\metricsize}p{\metricsize}p{\metricsize}p{\metricsize}p{\metricsize}p{\metricsize}|} 
\toprule
Method                                           & Metric      & \begin{sideways}DTD\end{sideways}        & \multicolumn{1}{|l|}{\begin{sideways}SVHN\end{sideways}} & \multicolumn{1}{l|}{\begin{sideways}Places365\end{sideways}} & \multicolumn{1}{l|}{\begin{sideways}CIFAR-10\end{sideways}} & \multicolumn{1}{l|}{\begin{sideways}MNIST\end{sideways}} & \multicolumn{1}{l|}{\begin{sideways}TIN\end{sideways}} & \begin{sideways}Average\end{sideways}     \\ 
\hline
\hline
% \multirow{3}{*}{\Longunderstack{\ours \\ Real \OOD}} & {\cellcolor{\fprcolor}}{\tiny FPR$\downarrow$}   & {\cellcolor{\fprcolor}} 60.50 & {\cellcolor{\fprcolor}} \textbf{42.54}              & {\cellcolor{\fprcolor}} 74.57                     & {\cellcolor{\fprcolor}} 83.80                     & {\cellcolor{\fprcolor}} 60.12                 & {\cellcolor{\fprcolor}} \textbf{71.06}               & {\cellcolor{\fprcolor}} 65.43  \\
%                                                  & {\cellcolor{\auroccolor}}{\tiny AUROC$\uparrow$} & {\cellcolor{\auroccolor}} 81.03 & {\cellcolor{\auroccolor}} \textbf{92.45}                & {\cellcolor{\auroccolor}} 79.71                     & {\cellcolor{\auroccolor}} 72.53                     & {\cellcolor{\auroccolor}} 86.22                 & {\cellcolor{\auroccolor}} 81.58               & {\cellcolor{\auroccolor}} 85.01  \\
%                                                  & {\cellcolor{\auprcolor}}{\tiny AUPR$\uparrow$}  & {\cellcolor{\auprcolor}} 86.31 & {\cellcolor{\auprcolor}} \textbf{87.60}                & {\cellcolor{\auprcolor}} 20.76                     & {\cellcolor{\auprcolor}} 72.36                     & {\cellcolor{\auprcolor}}  88.57                 & {\cellcolor{\auprcolor}} 82.20               & {\cellcolor{\auprcolor}} 72.96  \\ 
\multirow{3}{*}{\Longunderstack{\oursreal}} & {\cellcolor{\fprcolor}}{\tiny FPR$\downarrow$}   & {\cellcolor{\fprcolor}} {47.93} & {\cellcolor{\fprcolor}} \textbf{39.18}              & {\cellcolor{\fprcolor}} 72.31                     & {\cellcolor{\fprcolor}} 85.42                     & {\cellcolor{\fprcolor}} 35.99                 & {\cellcolor{\fprcolor}} {67.58}               & {\cellcolor{\fprcolor}} {58.07}  \\
                                                 & {\cellcolor{\auroccolor}}{\tiny AUROC$\uparrow$} & {\cellcolor{\auroccolor}} {89.1} & {\cellcolor{\auroccolor}} \textbf{93.25}                & {\cellcolor{\auroccolor}} 80.65                     & {\cellcolor{\auroccolor}}70.47                     & {\cellcolor{\auroccolor}} 94.01                 & {\cellcolor{\auroccolor}} {82.55}               & {\cellcolor{\auroccolor}} 85.01  \\
                                                 & {\cellcolor{\auprcolor}}{\tiny AUPR$\uparrow$}  & {\cellcolor{\auprcolor}} {93.45} & {\cellcolor{\auprcolor}} {88.48}                & {\cellcolor{\auprcolor}} 20.76                     & {\cellcolor{\auprcolor}} 68.66                     & {\cellcolor{\auprcolor}}  94.88                & {\cellcolor{\auprcolor}} 82.49              & {\cellcolor{\auprcolor}} 74.78  \\ 
\hline
\multirow{3}{*}{\Longunderstack{\oursfake}} & {\cellcolor{\fprcolor}}{\tiny FPR$\downarrow$}   & {\cellcolor{\fprcolor}} {51.28} & {\cellcolor{\fprcolor}} 46.43                & {\cellcolor{\fprcolor}} \textbf{71.9 }                    & {\cellcolor{\fprcolor}} \textbf{84.47}                     & {\cellcolor{\fprcolor}} {27.02}                  & {\cellcolor{\fprcolor}} 68.87              & {\cellcolor{\fprcolor}} {58.32}  \\
                                                 & {\cellcolor{\auroccolor}}{\tiny AUROC$\uparrow$} & {\cellcolor{\auroccolor}} {85.86} & {\cellcolor{\auroccolor}} 91.63                & {\cellcolor{\auroccolor}} \textbf{81.21}                     & {\cellcolor{\auroccolor}} \textbf{72.56}                     & {\cellcolor{\auroccolor}} {95.72}                 & {\cellcolor{\auroccolor}} 82.18               & {\cellcolor{\auroccolor}} {84.86}  \\
                                                 & {\cellcolor{\auprcolor}}{\tiny AUPR$\uparrow$}  & {\cellcolor{\auprcolor}} 86.58 & {\cellcolor{\auprcolor}} \textbf{90.34}                & {\cellcolor{\auprcolor}} \textbf{21.07 }                   & {\cellcolor{\auprcolor}} \textbf{74.34}                     & {\cellcolor{\auprcolor}} {96.26}                 & {\cellcolor{\auprcolor}} 82.46               & {\cellcolor{\auprcolor}} 75.17  \\ 
\hline
\multirow{3}{*}{\Longunderstack{\ours \\ Mixed \OOD}} & {\cellcolor{\fprcolor}}{\tiny FPR$\downarrow$}   & {\cellcolor{\fprcolor}} \textbf{42.55} & {\cellcolor{\fprcolor}} 41.46                & {\cellcolor{\fprcolor}} 72.7                   & {\cellcolor{\fprcolor}} {85.74}                     & {\cellcolor{\fprcolor}} \textbf{24.22}                  & {\cellcolor{\fprcolor}}\textbf{66.97}  & {\cellcolor{\fprcolor}} \textbf{55.60}  \\
                                                 & {\cellcolor{\auroccolor}}{\tiny AUROC$\uparrow$} & {\cellcolor{\auroccolor}} \textbf{90.92} & {\cellcolor{\auroccolor}}  93.12               & {\cellcolor{\auroccolor}} {80.39}                     & {\cellcolor{\auroccolor}} 69.97                     & {\cellcolor{\auroccolor}} \textbf{96.19}                 & {\cellcolor{\auroccolor}}\textbf{82.72}             & {\cellcolor{\auroccolor}} \textbf{85.55}  \\
                                                 & {\cellcolor{\auprcolor}}{\tiny AUPR$\uparrow$}  & {\cellcolor{\auprcolor}}\textbf{94.63} & {\cellcolor{\auprcolor}} {88.97}                & {\cellcolor{\auprcolor}} 19.26                     & {\cellcolor{\auprcolor}} 67.51                     & {\cellcolor{\auprcolor}} \textbf{96.69}                 & {\cellcolor{\auprcolor}}\textbf{82.61}              & {\cellcolor{\auprcolor}} 74.94  \\ 
\hline
% 66.97 AUC 82.72 AUPIN 82.61
\bottomrule
\end{tabular}

\caption {{Comparison of our method's variants on CIFAR-100 dataset. }}
\label{tab:mixed_cifar100}

\end{table}
